# Supplementary material for: Outlier-Robust Estimation: Hardness, Minimally Tuned Algorithms, and Applications
Source: arXiv:2007.15109 source file (2021-07-02)
Supplement: Supplementary file 1 [file appendix-bisection.tex]

%!TEX root = ../main.tex

\section{$\fitbisection$ algorithm}\label{app:alg-fitbisection}

\gncfree's subroutine $\fitbisection$ is presented in Algorithm~\ref{alg:fitcdf}.
$\fitbisection$ aims to improve the inlier noise $\inthr$ initial guess trying when the noise upper bound $\noiseupbound$ scores a bad $\chi^2$ fit.
The algorithm initialize the upper and lower bound for $\inthr$ with resp., $\noiseupbound$ and $\noiselowbound$ and evaluates the fitness score after the outlier rejection (lines~\ref{line:bisection-init}-\ref{line:bisection-initscore}).
Until the score it not close to the target value $\gamma$, it performs a binary search, stopping if 
(i) the fitness score does not improve across iterations (line~\ref{line:bisection-stop1}), or 
(iii) the spread $(a-b)/a$ is too small (line~\ref{line:bisection-stop2}).
It then returns the next $\inthr$ to test.

%%%%%%%%%%
%!TEX root = ../main.tex

\begin{algorithm}[h]\label{alg:bisection}
	\caption{\mbox{$\fitbisection$ (\gncfree's subroutine).}}
	\SetAlgoLined
	\KwIn{\mbox{Measurements $\vy_i,\;\forall i\in\measSet$;} $\noiseupbound\geq 0$; $\noiselowbound \geq 0$;\mbox{Target critical value $\gamma$}}
	\KwOut{\mbox{Initial guess for $\inthr$}}
  \BlankLine
  $a = c = \noiseupbound;\> b=\noiselowbound$\label{line:bisection-init}\;
  $(\vxx,\inset) = \gncalg(\vy, c);\> s = \fitChi(\vres(\vy_\inset,\vxx), d)$\label{line:bisection-initscore}\; 
  $e = s/\gamma$\;
  \While{$e > 1.1$ {\bf or} $e < 0.9$}{
    $c = (a+b)/2$\;
    $(\vxx,\inset) = \gncalg(\vy, c);\> s = \fitChi(\vres(\vy_\inset,\vxx), d)$\;
    \lIf{$|s/\gamma - e| < \num{1e-3}$\label{line:bisection-stop1}}{
      \KwBreak%\Return{$c$.}\;
    }
    \lElseIf{$s/\gamma > 1.1$}{
      $a = c$
    }\lElseIf{$s/\gamma > 0.9$}{
      $b = c$
    }
    \lIf{$(a-b)/a < 0.1$}{
      \KwBreak\label{line:bisection-stop2}%\Return{$c$.}
    }
    $e = s/\gamma$\;
  }
  % \mbox{$\inlierNoise \!=\! }\label{line:bisection-inlierguess-update}\;
  \Return{$\displaystyle\max_{i\; \in \; \inset}\;\{\res(\vy_{i},\vxx) \;\text{s.t.}\;\res(\vy_{i},\vxx) \!<\!c\}\label{line:bisection-return}$.}
\end{algorithm}
%%%%%%%%%%
