# Supplementary material for: Outlier-Robust Estimation: Hardness, Minimally Tuned Algorithms, and Applications
Source: arXiv:2007.15109 source file (2021-07-02)
Supplement: Supplementary file 2 [file appendix-bound-slam.tex]

%!TEX root = main.tex

\subsection{Bound for SLAM}
\label{sec:proof:bound-slam}

Let us consider the following SLAM  problem (Pose Graph Optimization):
\bea
\min_{\MT_i\in\SE{d}} 
\sum_{(i,j) \in \calE_o} \| \MT_j - \MT_i \bar{\MT}_{ij} \|^2_\Omega
+ \hspace{-4mm}
\sum_{(i_k,j_k) \in \calE_{lc}} \| \MT_{j_k} - \MT_{i_k} \bar{\MT}_{k} \|^2_\Omega
\eea
where $\calE_o$ are the (reliable) odometry edges, while $\calE_{lc}$ are the (possibly unreliable) loop closures. Note that we indexed the loop closures using $k = 1,\ldots,|\calE_{lc}|$, such that the $k$-th loop closure connects poses $(i_k,j_k)$.

Let us define the set function:
\bea
f(\calS) = 
\min_{\MT_i\in\SE{d}} 
\sum_{(i,j) \in \calE_o} \| \MT_j - \MT_i \bar{\MT}_{ij} \|^2_\Omega
+\hspace{-6mm}
\sum_{(i_k,j_k) \in \calE_{lc} \setminus\calS}\hspace{-4mm}\| \MT_{j_k} - \MT_{i_k} \bar{\MT}_{k} \|^2_\Omega
\eea
and it's normalized version:
\bea
\bar{f}(\calS) = f(\emptyset) - f(\calS)
\eea
which is also positive ($\bar{f}(\calS) \geq 0, \forall \calS \subseteq \calE_{lc}$) and non-decreasing ($\bar{f}(\calS_1) \leq \bar{f}(\calS_2), \forall \calS_1 \subseteq \calS_2 \subseteq \calE_{lc}$, since $f(\calS_1) \geq f(\calS_2), \forall \calS_1 \subseteq \calS_2 \subseteq \calE_{lc}$). 
Eventually, we would like to solve:
\beq
\max_{|\calS|=\beta} \bar{f}(\calS)
\eeq
which looks for the set $\calS$ that makes $f(\calS)$ as small as possible.

Finally, define the marginal gain:
\bea
\bar{f}(\{s\}|\calS) \triangleq \bar{f}(\calS \cup \{s\})  - \bar{f}(\calS) =  {f}(\calS) - {f}(\calS \cup \{s\})
\eea

Our goal now is to compute a good and computationally-inexpensive upper-bound for $\bar{f}(\{s\}|\calS)$, which can be used in the Lazy greedy algorithm. In particular:
\bit
\item we want to avoid computing ${f}(\calS \cup \{s\})$ at each iteration of the greedy.
\item we can leverage the knowledge of ${f}(\calS)$ which has been computed at the previous iteration.
\eit

We also remark that computing an upper-bound for $\bar{f}(\{s\}|\calS)$ for a fixed ${f}(\calS)$ is the same as computing a lower-bound for ${f}(\calS \cup \{s\})$.
% Moreover, we are looking for a bound tighter than ${f}(\calS \cup \{s\}) \leq {f}(\calS)$

Therefore in the following we compute a lower bound for ${f}(\calS \cup \{s\})$. 
For this purpose, we note that the original cost function can be written as:
\bea
\min_{\MT_i\in\SE{d}} 
\sum_{(i_k,j_k) \in \calE_{lc}} 
\left(\| \MT_{j_k} - \MT_{i_k} \bar{\MT}_{k} \|^2_\Omega
+
\sum_{(i,j) \in \calE^k_o} \frac{1}{n_{ij}(\calE_{lc})} \| \MT_j - \MT_i \bar{\MT}_{ij} \|^2_\Omega
\right)
\eea
where $n_{ij}(\calE_{lc})$ is the number of loops the odometry edge is involved in, within the graph with loop closures $\calE_{lc}$. Similarly:
\bea
f(\calS) = 
\min_{\MT_i\in\SE{d}} %\hspace{-1cm}
	\sum_{(i_k,j_k) \in \calS } 
\left(
\sum_{(i,j) \in \calE^k_o} \frac{1}{n_{ij}(\calE_{lc})} \| \MT_j - \MT_i \bar{\MT}_{ij} \|^2_\Omega
\right)
\\
+ \hspace{-4mm}\sum_{(i_k,j_k) \in \calE_{lc} \setminus \calS} 
\left(\| \MT_{j_k} - \MT_{i_k} \bar{\MT}_{k} \|^2_\Omega
+ \hspace{-4mm}
\sum_{(i,j) \in \calE^k_o} \frac{1}{n_{ij}(\calE_{lc})} \| \MT_j - \MT_i \bar{\MT}_{ij} \|^2_\Omega
\right)
\\
\geq 
\\
\sum_{(i_k,j_k) \in \calS} 
\min_{\MT_i\in\SE{d}}
\left(
\sum_{(i,j) \in \calE^k_o} \frac{1}{n_{ij}(\calE_{lc})} \| \MT_j - \MT_i \bar{\MT}_{ij} \|^2_\Omega
\right)
\\
+ \hspace{-4mm}\sum_{(i_k,j_k) \in \calE_{lc} \setminus \calS} 
\min_{\MT_i\in\SE{d}}
\left(\| \MT_{j_k} - \MT_{i_k} \bar{\MT}_{k} \|^2_\Omega
+ \hspace{-4mm}
\sum_{(i,j) \in \calE^k_o} \frac{1}{n_{ij}(\calE_{lc})} \| \MT_j - \MT_i \bar{\MT}_{ij} \|^2_\Omega
\right)
\\
=
\\
\hspace{-4mm}\sum_{(i_k,j_k) \in \calE_{lc} \setminus \calS} 
\min_{\MT_i\in\SE{d}}
\left(\| \MT_{j_k} - \MT_{i_k} \bar{\MT}_{k} \|^2_\Omega
+ \hspace{-4mm}
\sum_{(i,j) \in \calE^k_o} \frac{1}{n_{ij}(\calE_{lc})} \| \MT_j - \MT_i \bar{\MT}_{ij} \|^2_\Omega
\right)
\eea
Therefore we can compute the following (independent) quantities, for each $s \in \calE_{lc}$:
\bea
b_k \doteq \min_{\MT_i\in\SE{d}}
\left(\| \MT_{j_k} - \MT_{i_k} \bar{\MT}_{k} \|^2_\Omega
+ \hspace{-4mm}
\sum_{(i,j) \in \calE^k_o} \frac{1}{n_{ij}(\calE_{lc})} \| \MT_j - \MT_i \bar{\MT}_{ij} \|^2_\Omega
\right) 
\eea
And the desired lower bound for ${f}(\calS \cup \{s\})$
\bea
{f}(\calS \cup \{s\}) \geq \sum_{k\in \calS \cup \{s\}} b_k
\eea
Note that
\bit
\item $b_k$ must be computed only once, at the beginning of the greedy
\item each computation of $b_k$ involves an optimization over a single cycle, which is faster than optimizing over the entire graph. 
\eit

We also expect that outliers have large $b_k$ since they do not agree with the odometry and produce large errors even along the cycle they create in the graph, while inliers have small $b_k$ since they mostly agree with the odometry.
