# Supplementary material for: Outlier-Robust Estimation: Hardness, Minimally Tuned Algorithms, and Applications
Source: arXiv:2007.15109 source file (2021-07-02)
Supplement: Supplementary file 3 [file supp_2-view.tex]

%!TEX root = supplemental.tex
\newpage
\clearpage
\subsection{Supplemental for  Robust Two-view Geometry}
\label{sec:supp_view}

\input{supp_fig-2view}
